# Supplementary material for: Quantum tops at circular lepton colliders
Source: arXiv:2404.08049 ancillary file (2024-08-30)
Supplement: Supplementary file 1 [file 365_constraints.pdf]

## 1 SMEFT constraints for $e^+e^-$ at 365 GeV

In this additional section we collect all 2D exclusion regions for the simulated analysis of Section 7.3, for the  $e^+e^-$  circular collider operating at  $\sqrt{s} = 365$  GeV.

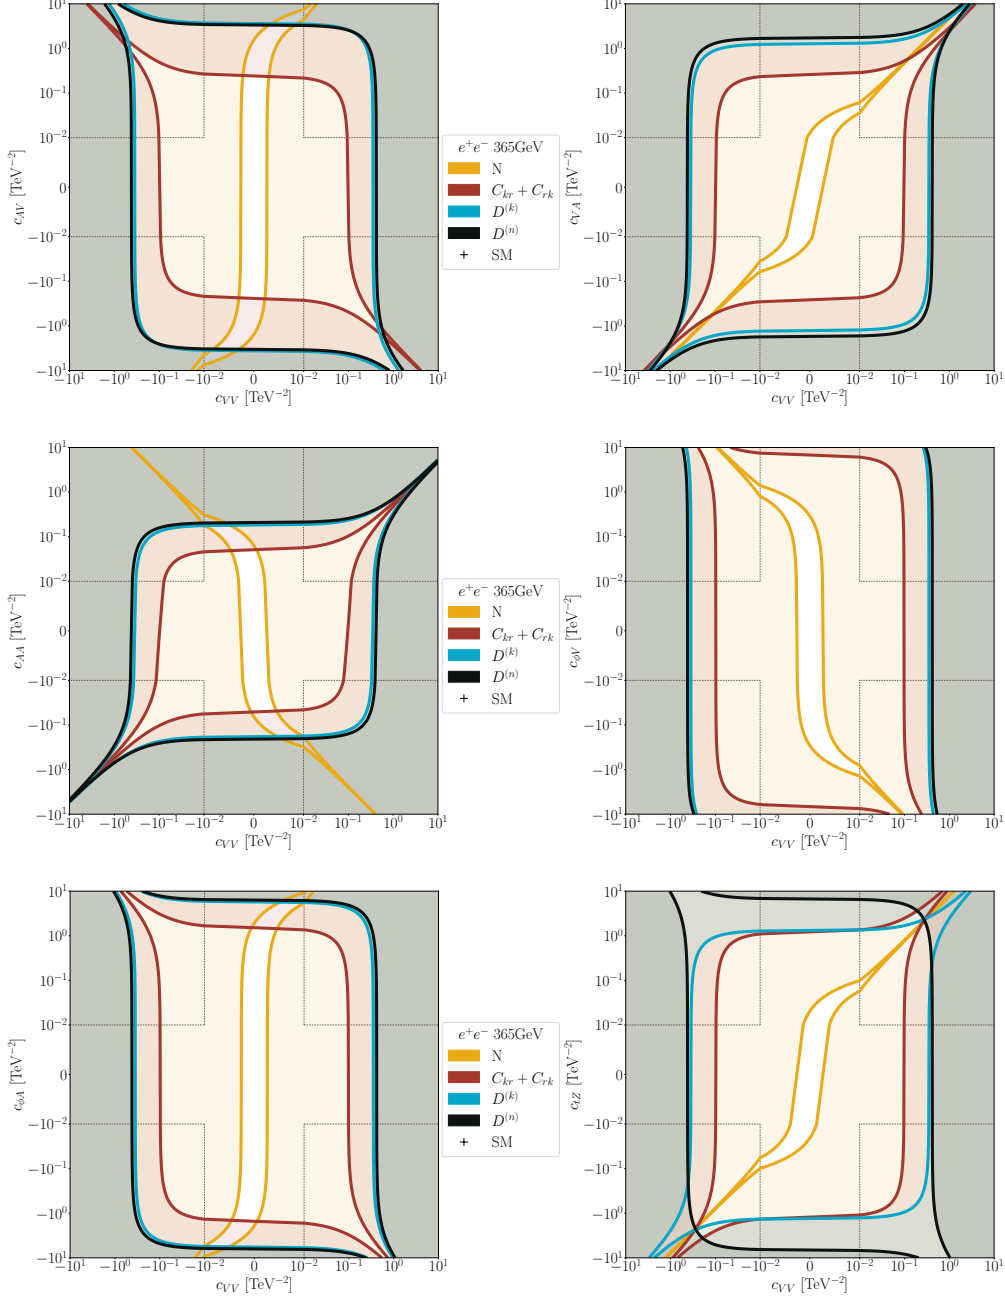

**Figure 1:** Same as in the figure 12 in Sec. 7.3 of the main paper, for the pairs  $(c_{VV}, c_{AV})$ ,  $(c_{VV}, c_{VA})$ ,  $(c_{VV}, c_{AA})$ ,  $(c_{VV}, c_{\phi V})$ ,  $(c_{VV}, c_{\phi A})$ ,  $(c_{VV}, c_{tZ})$ .

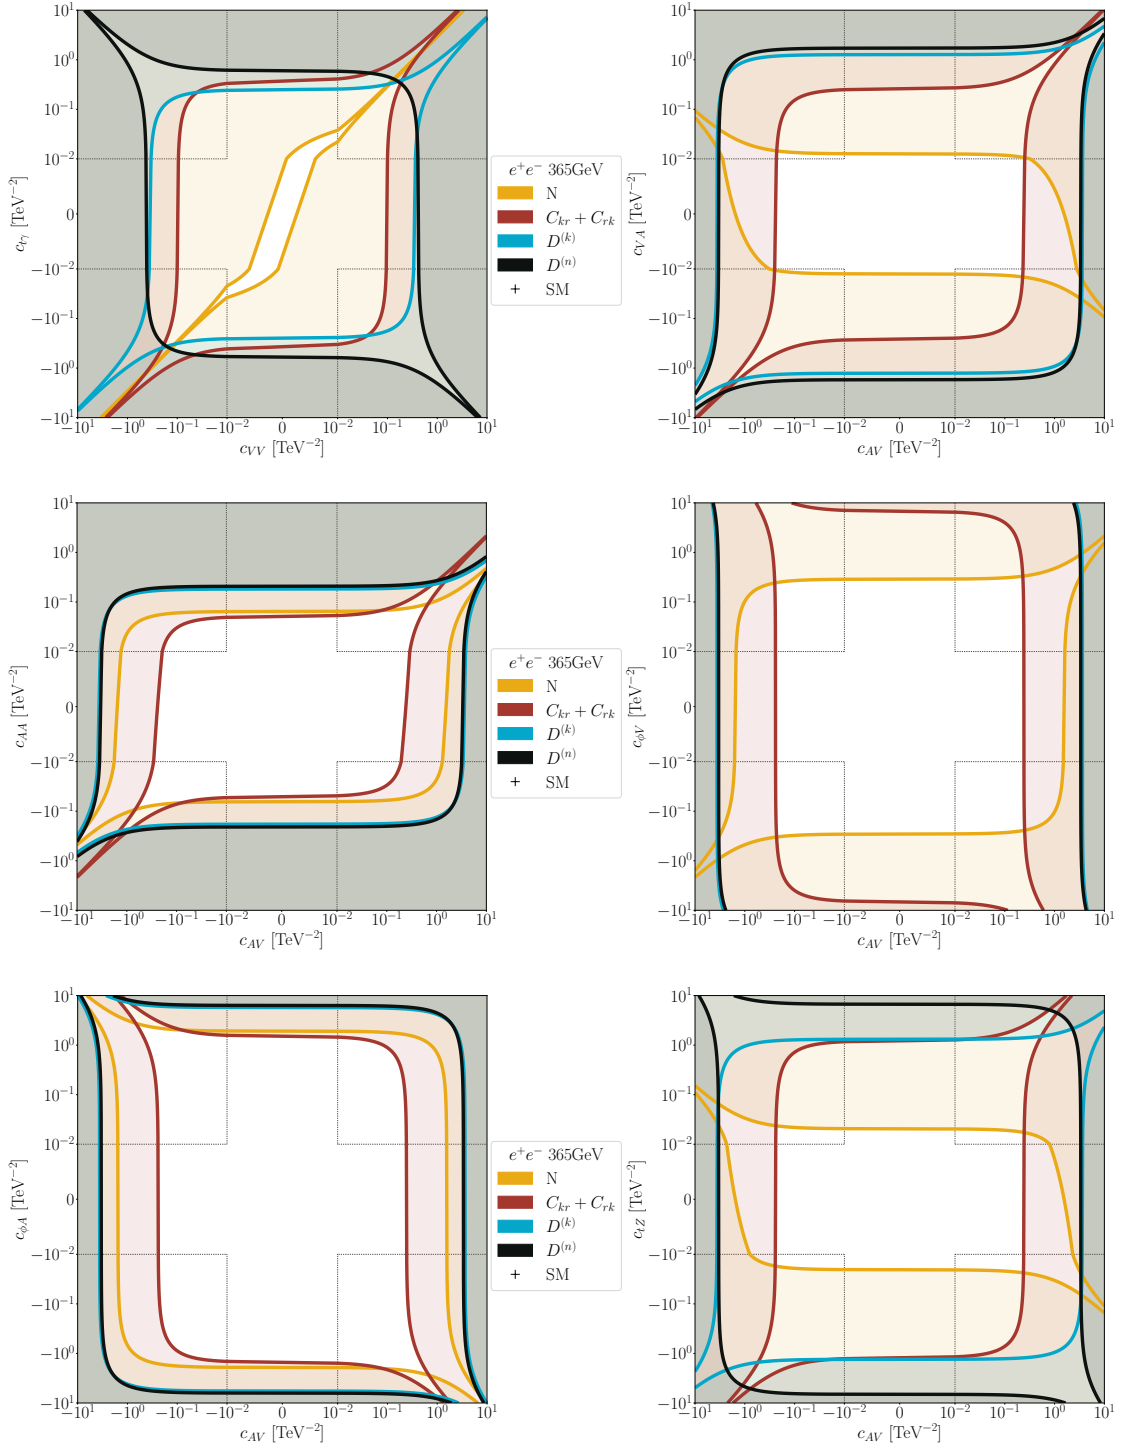

**Figure 2:** Same as in the figure 12 in Sec. 7.3 of the main paper, for the pairs  $(c_{VV}, c_{t\gamma})$ ,  $(c_{AV}, c_{VA})$ ,  $(c_{AV}, c_{AA})$ ,  $(c_{AV}, c_{\phi V})$ ,  $(c_{AV}, c_{\phi A})$ ,  $(c_{AV}, c_{tZ})$ .

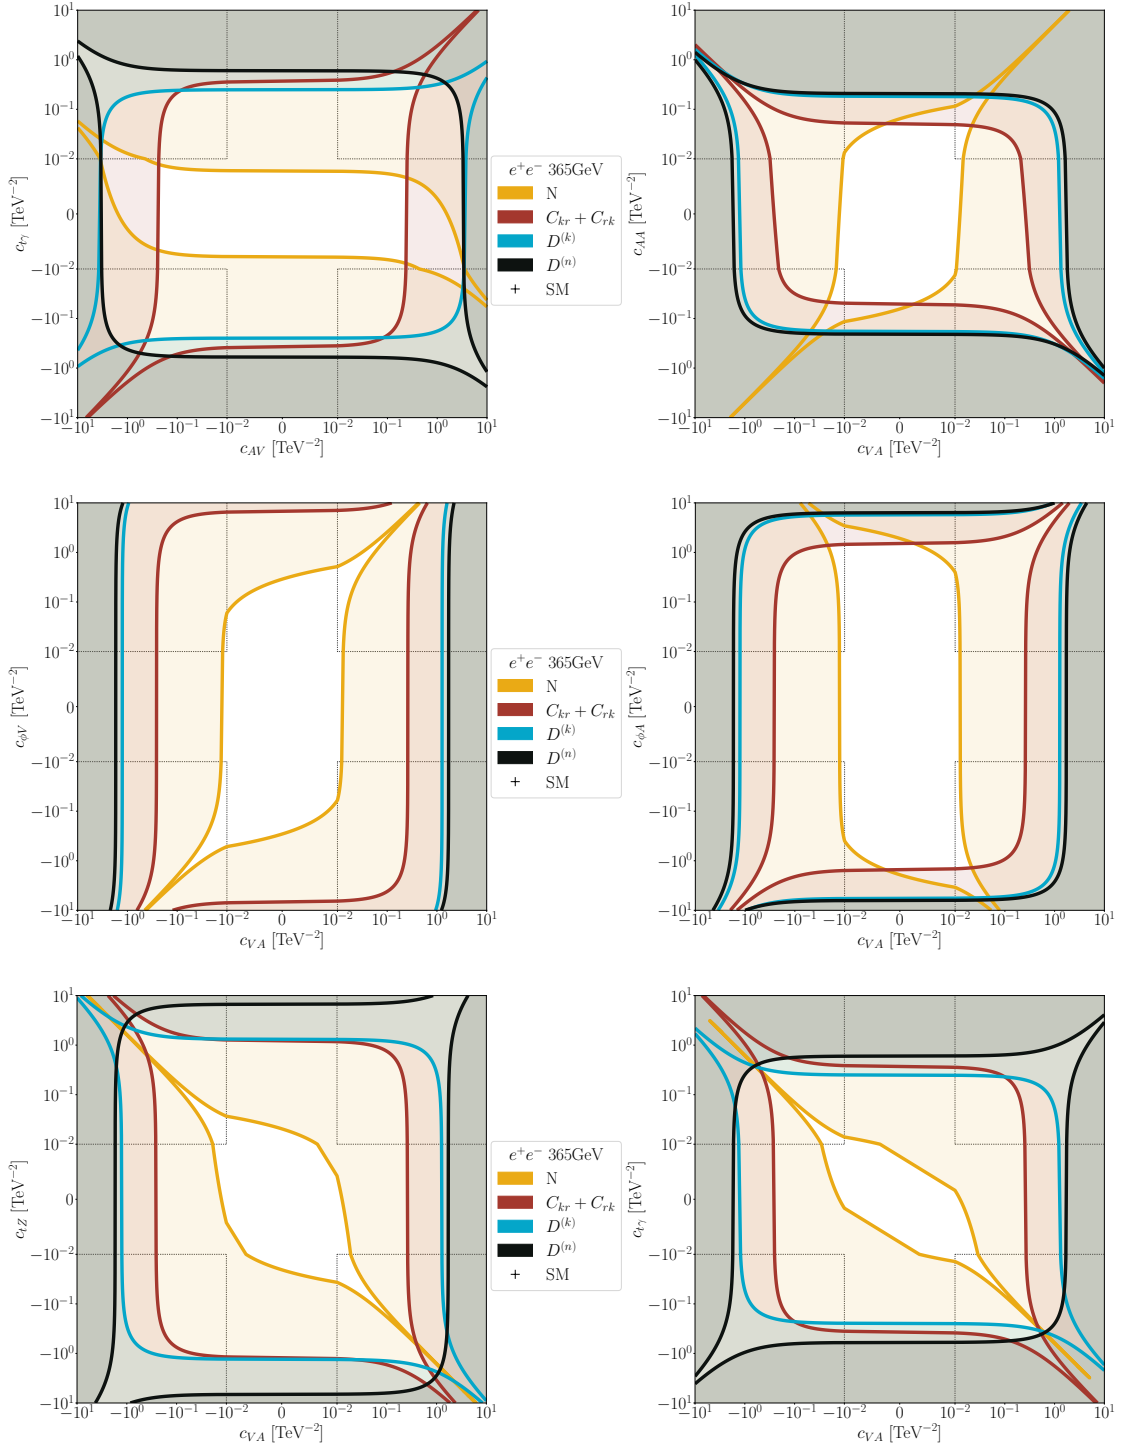

**Figure 3:** Same as in the figure 12 in Sec. 7.3 of the main paper, for the pairs  $(c_{AV}, c_{t\gamma})$ ,  $(c_{VA}, c_{AA})$ ,  $(c_{VA}, c_{\phi V})$ ,  $(c_{VA}, c_{\phi A})$ ,  $(c_{VA}, c_{tZ})$ ,  $(c_{VA}, c_{t\gamma})$ .

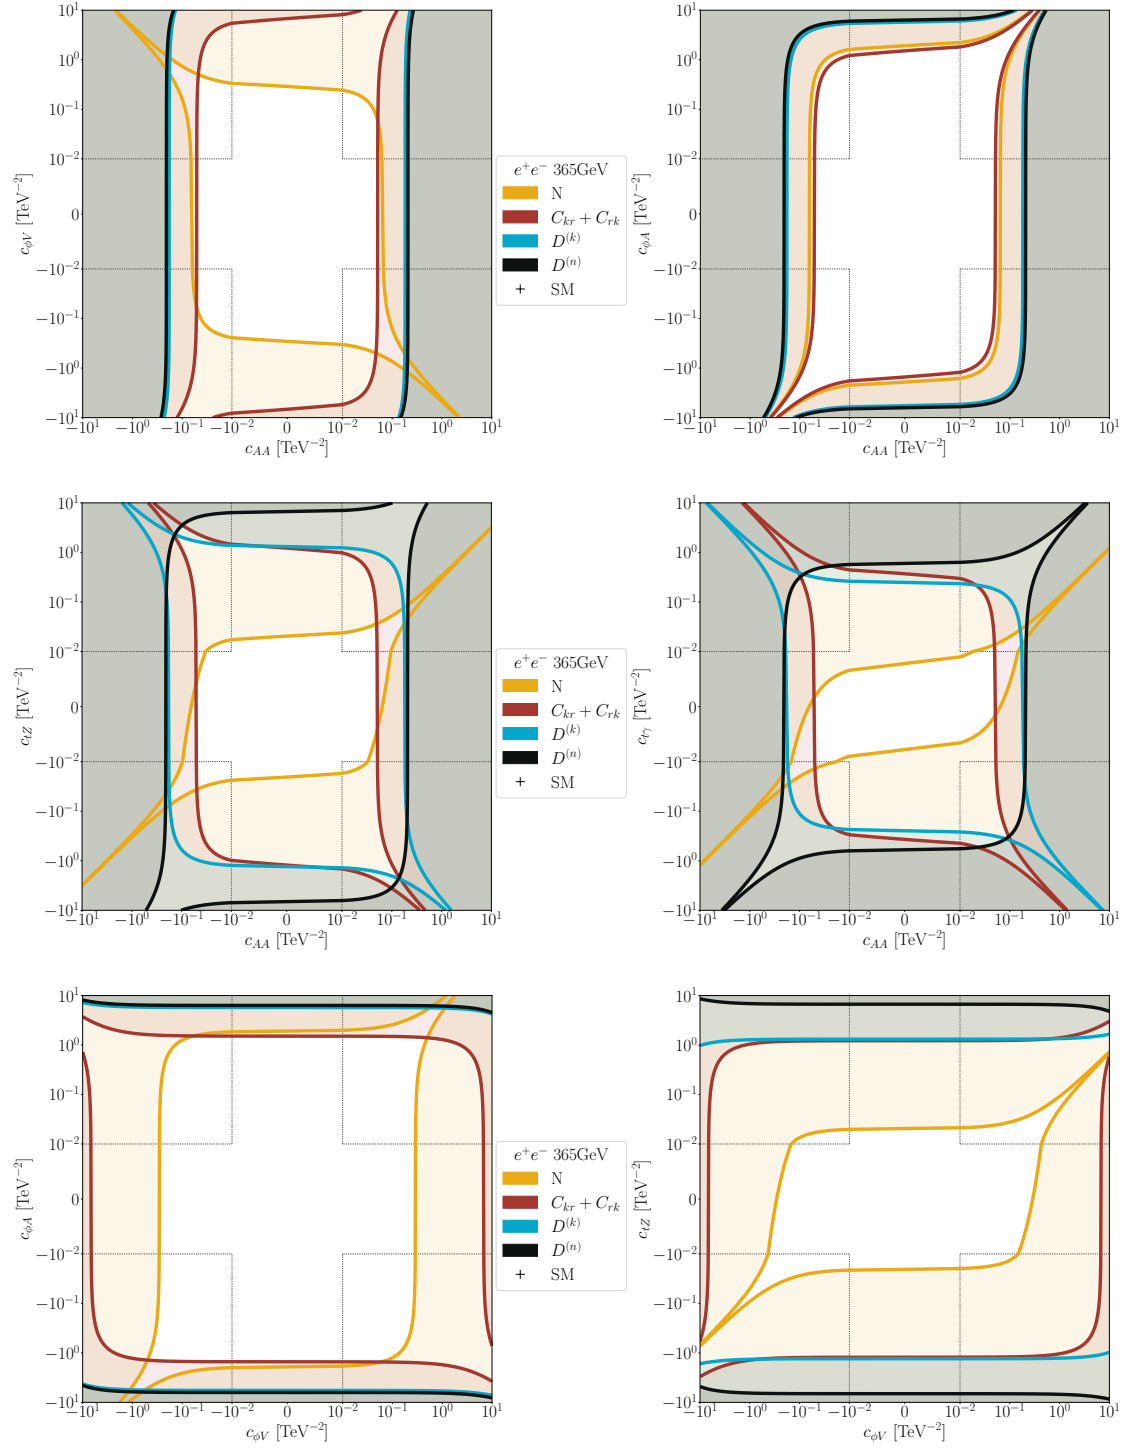

**Figure 4:** Same as in the figure 12 in Sec. 7.3 of the main paper, for the pairs  $(c_{AA}, c_{\phi V})$ ,  $(c_{AA}, c_{\phi A})$ ,  $(c_{AA}, c_{tZ})$ ,  $(c_{AA}, c_{t\gamma})$ ,  $(c_{\phi V}, c_{\phi A})$ ,  $(c_{\phi V}, c_{tZ})$ .



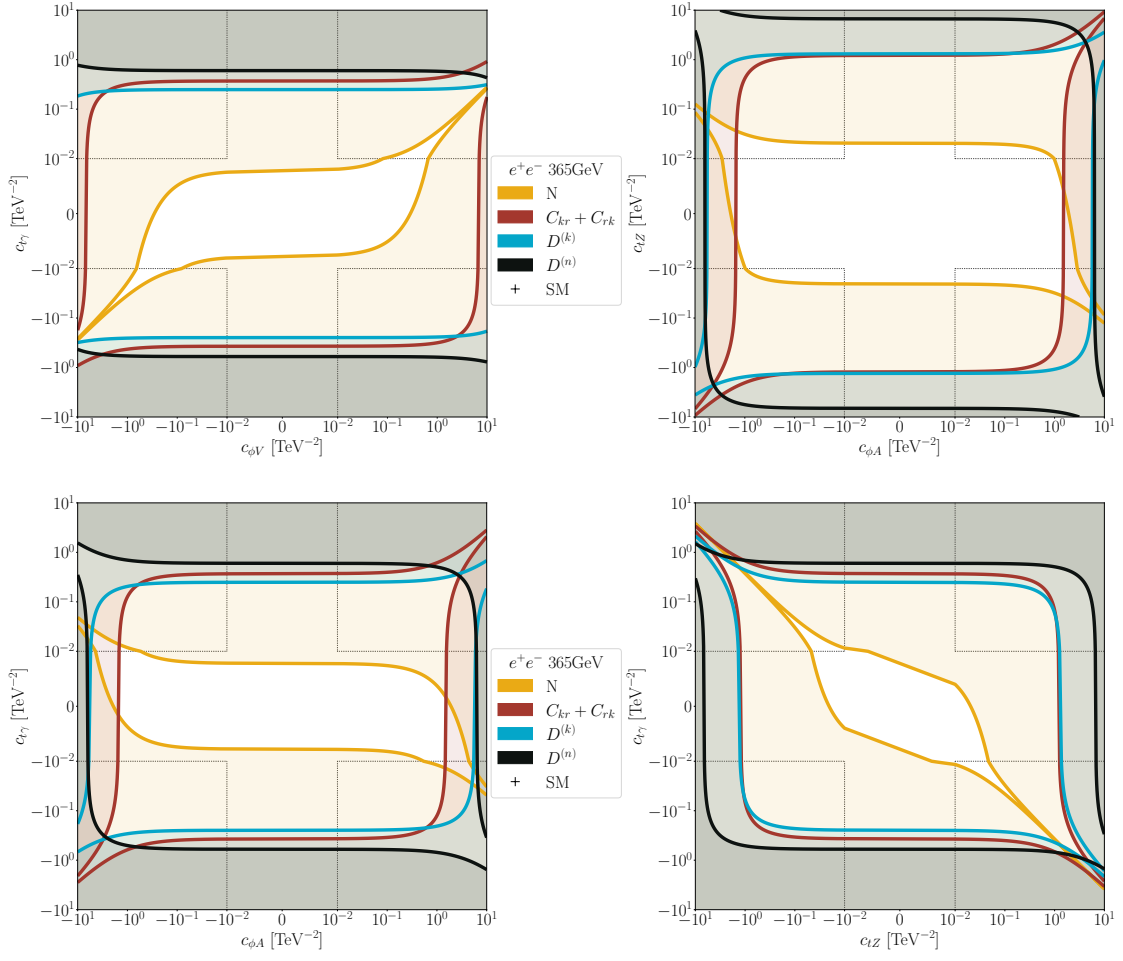

**Figure 5:** Same as in the figure 12 in Sec. 7.3 of the main paper, for the pairs  $(c_{\phi V}, c_{t\gamma})$ ,  $(c_{\phi A}, c_{tZ})$ ,  $(c_{\phi A}, c_{t\gamma})$ ,  $(c_{tZ}, c_{t\gamma})$ .
