# Supplementary material for: Quantum tops at circular lepton colliders
Source: arXiv:2404.08049 ancillary file (2024-08-30)
Supplement: Supplementary file 2 [file Energy_scan.pdf]

## SMEFT constraints for the lepton energy scan

In this Section we collect all 2D exclusion regions for the lepton energy scan we discussed in Section 7.5 of the main article.

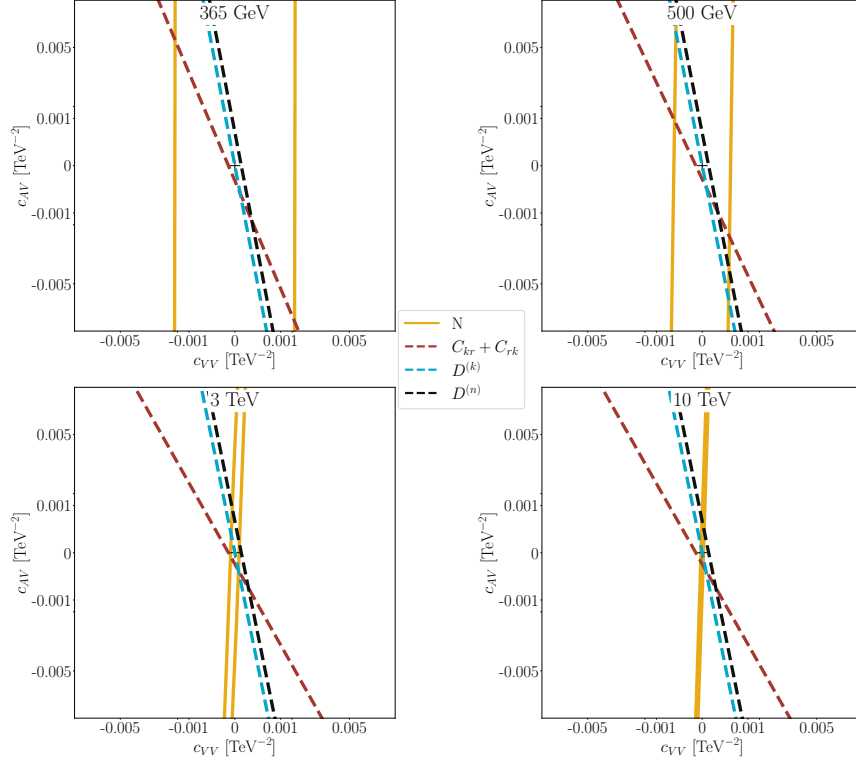

**Figure 1:** Exclusion plot for the couple of coefficient  $(c_{VV}, c_{AV})$  varying  $\sqrt{s}$ .

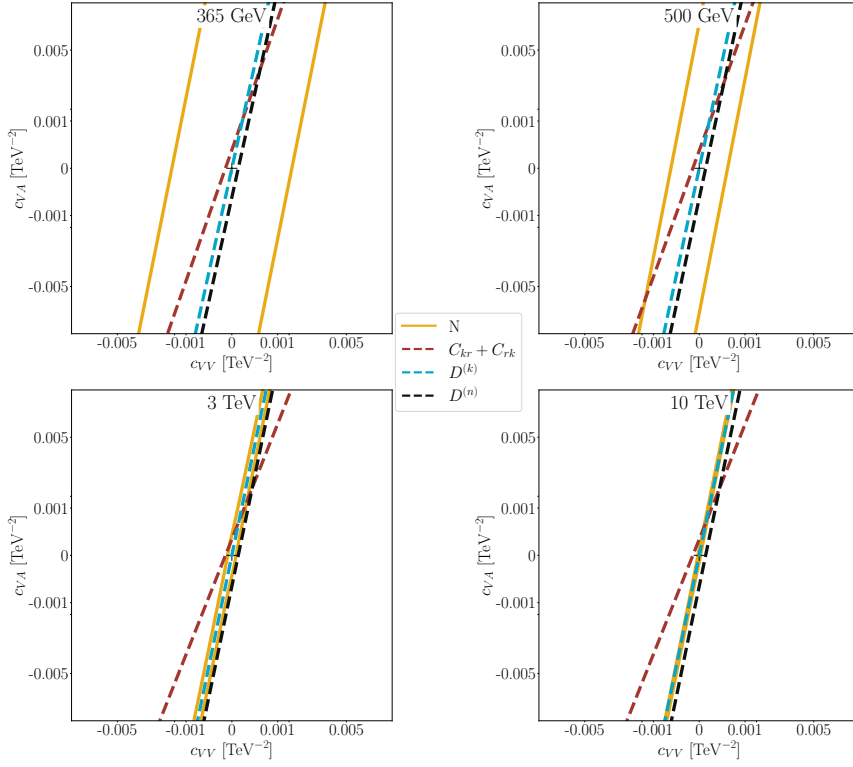

**Figure 2:** Exclusion plot for the couple of coefficient  $(c_{VV}, c_{VA})$  varying  $\sqrt{s}$ .

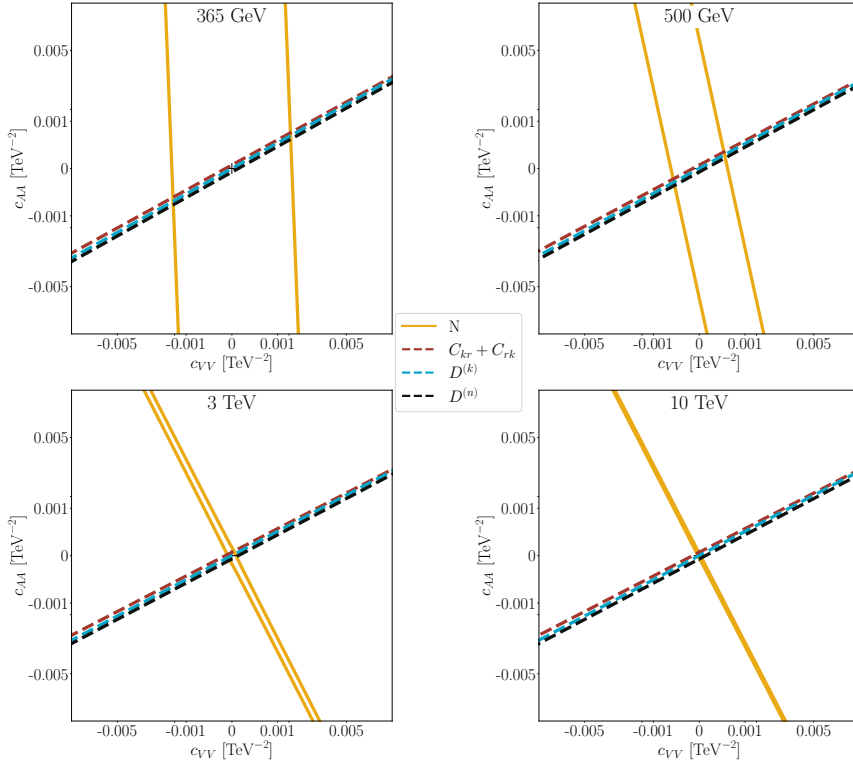

**Figure 3:** Exclusion plot for the couple of coefficient  $(c_{VV}, c_{AA})$  varying  $\sqrt{s}$ .

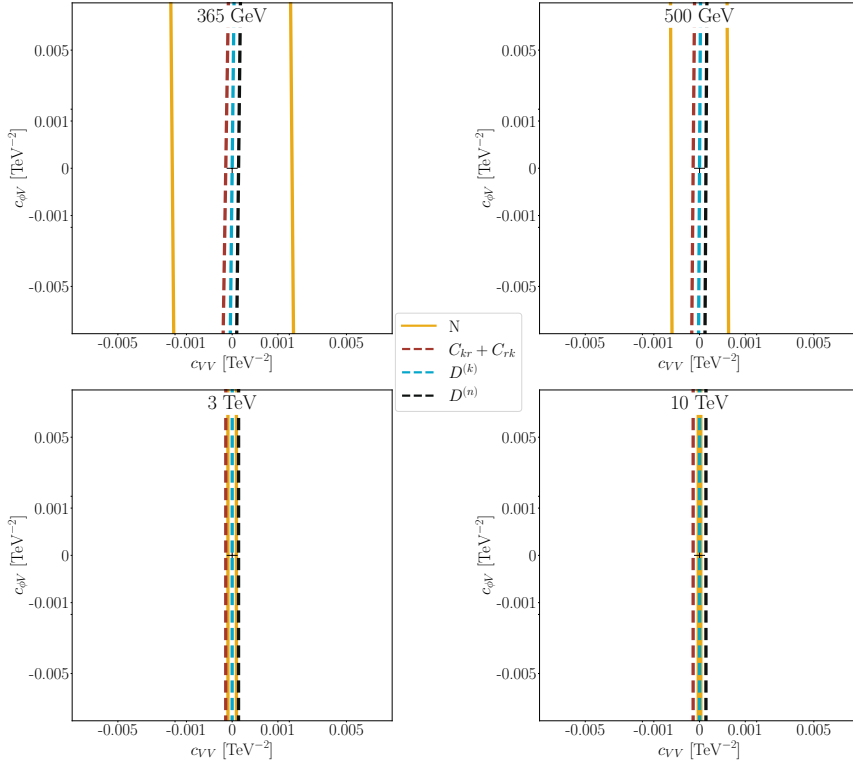

**Figure 4:** Exclusion plot for the couple of coefficient  $(c_{VV}, c_{\phi V})$  varying  $\sqrt{s}$ .

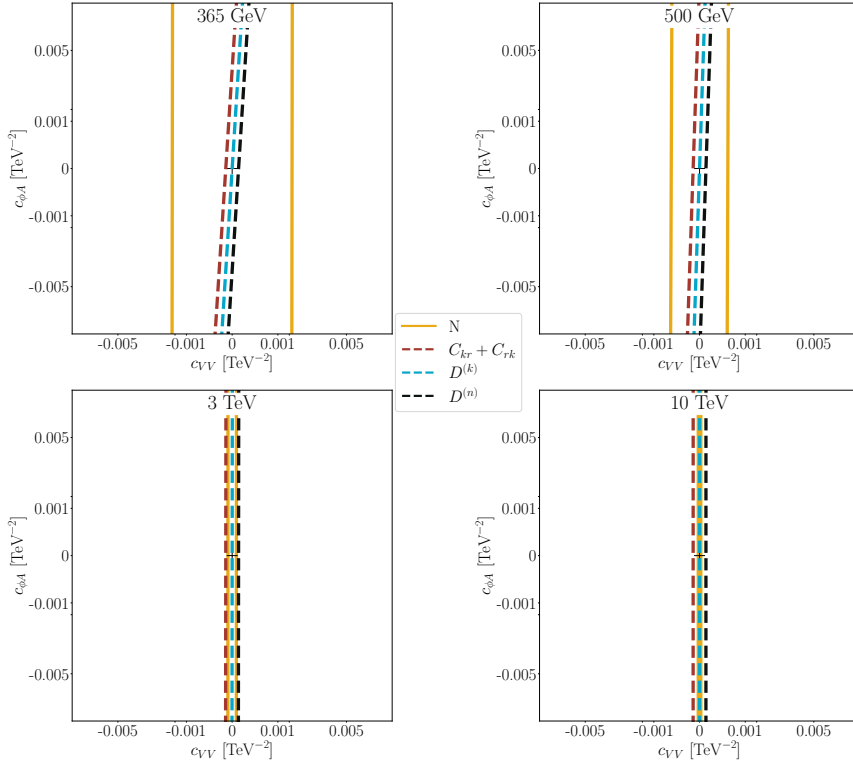

**Figure 5:** Exclusion plot for the couple of coefficient  $(c_{VV}, c_{\phi A})$  varying  $\sqrt{s}$ .

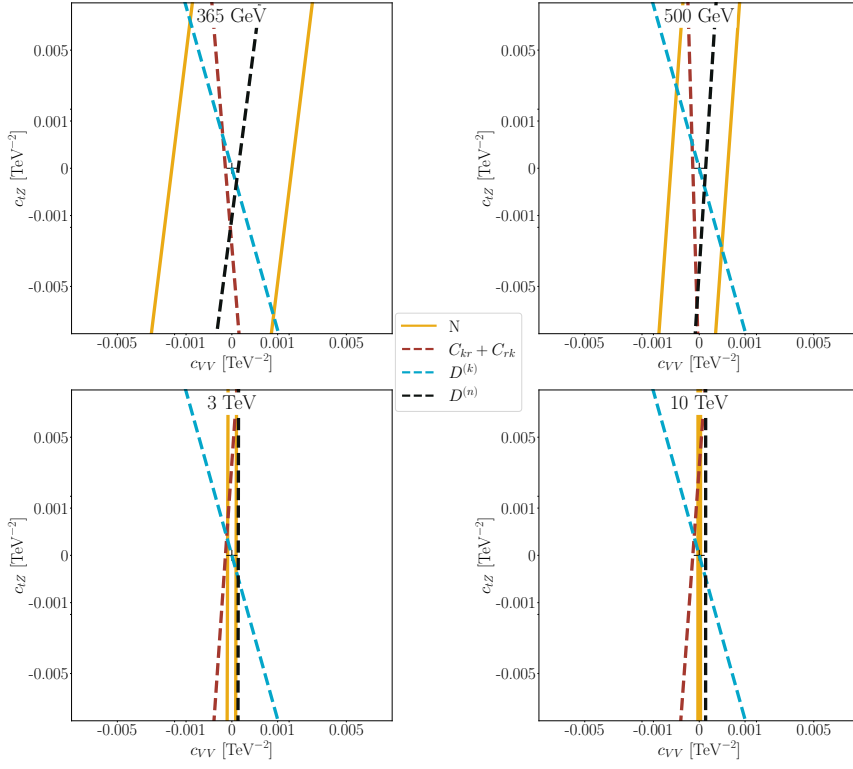

**Figure 6:** Exclusion plot for the couple of coefficient  $(c_{VV}, c_{tZ})$  varying  $\sqrt{s}$ .

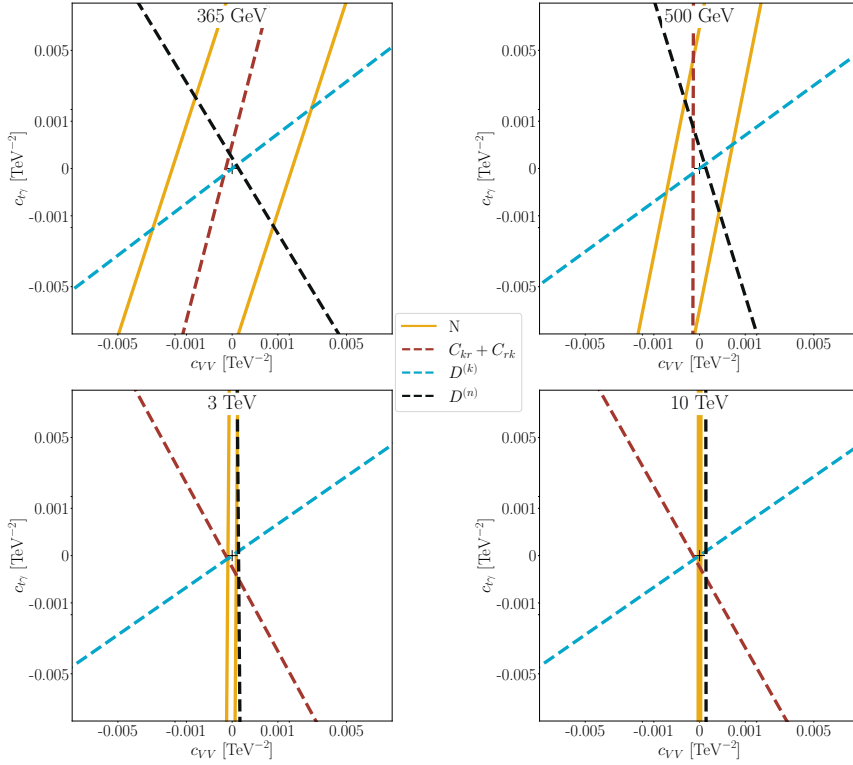

**Figure 7:** Exclusion plot for the couple of coefficient  $(c_{VV}, c_{t\gamma})$  varying  $\sqrt{s}$ .

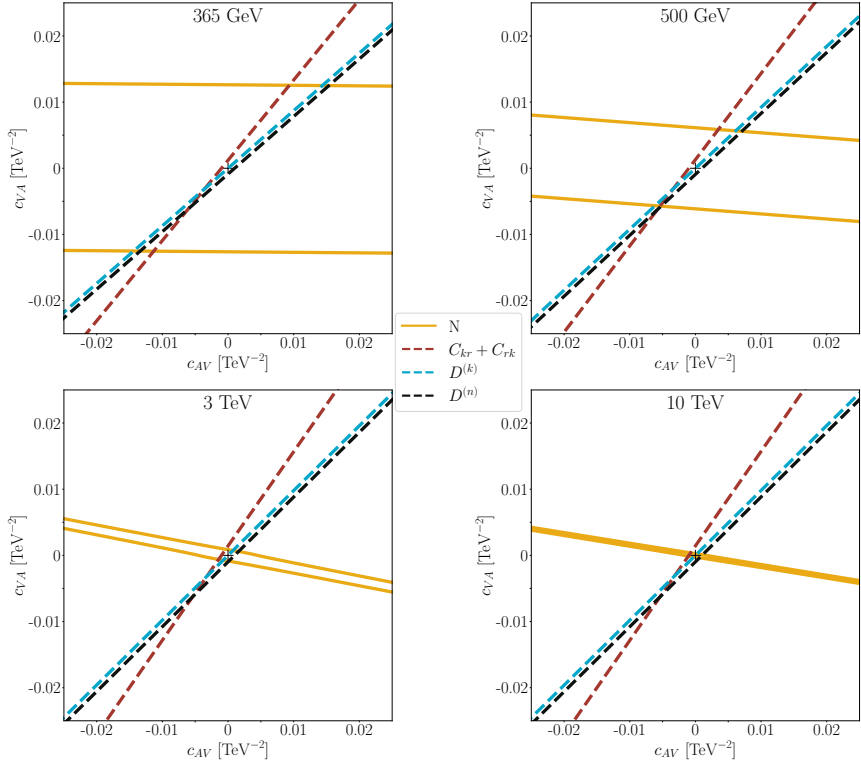

**Figure 8:** Exclusion plot for the couple of coefficient  $(c_{AV}, c_{VA})$  varying  $\sqrt{s}$ .

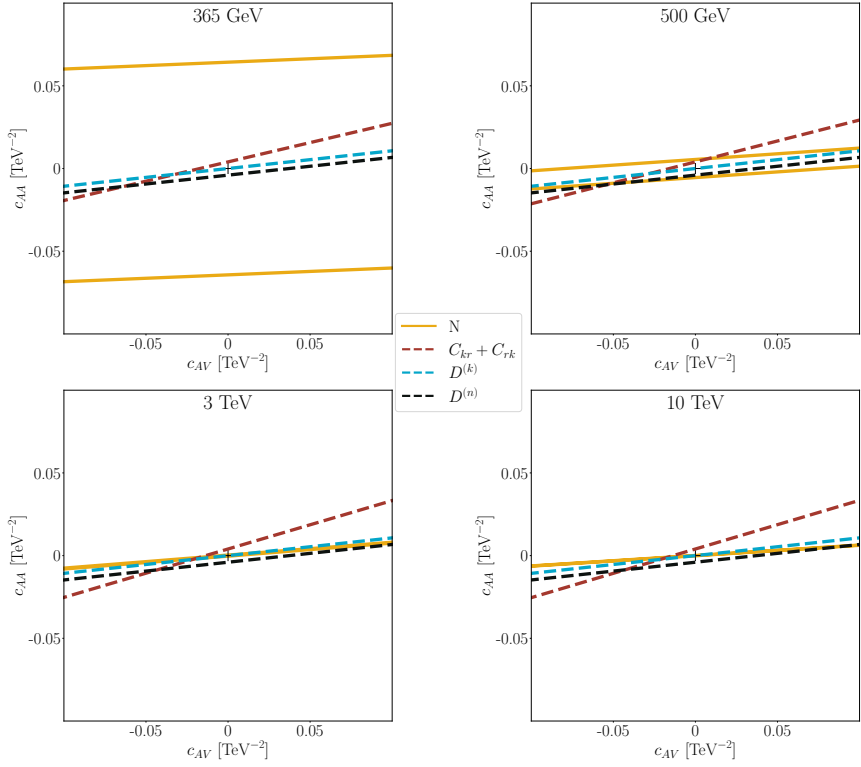

**Figure 9:** Exclusion plot for the couple of coefficient  $(c_{AV}, c_{AA})$  varying  $\sqrt{s}$ .

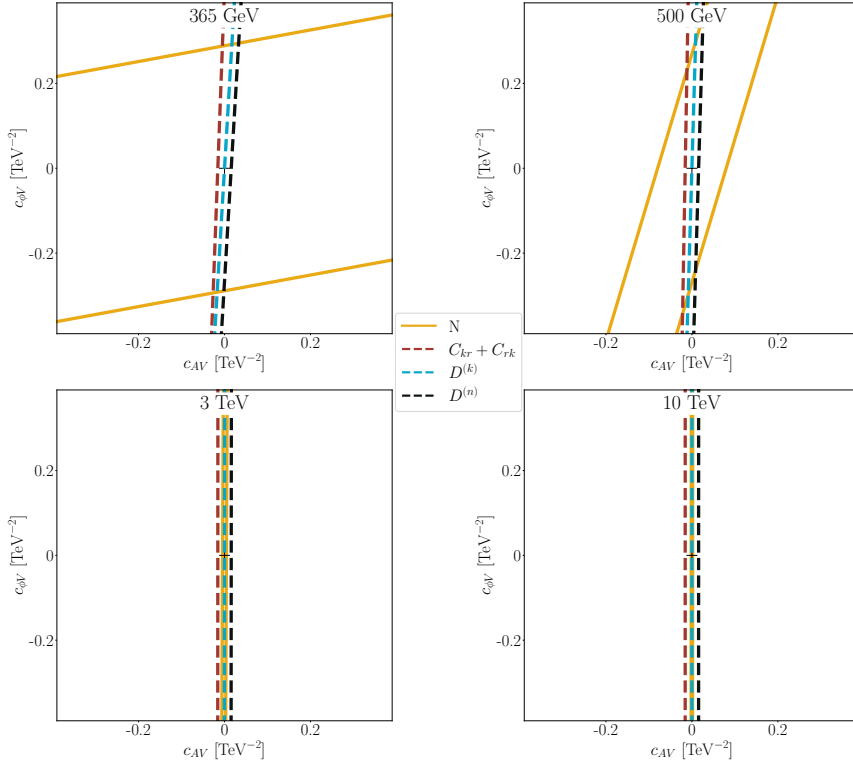

**Figure 10:** Exclusion plot for the couple of coefficient  $(c_{AV}, c_{\phi V})$  varying  $\sqrt{s}$ .

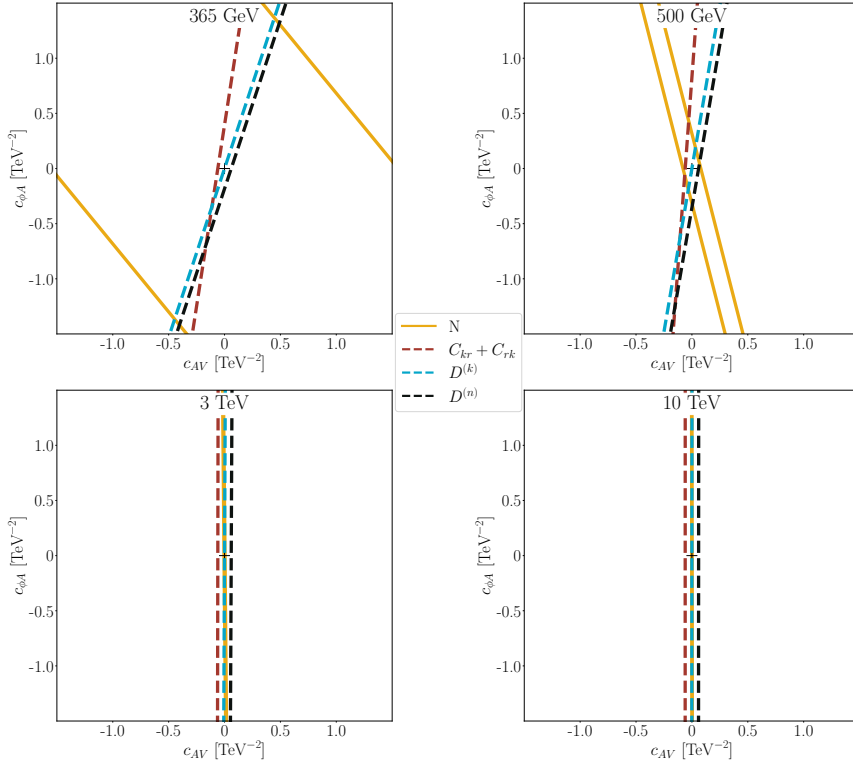

**Figure 11:** Exclusion plot for the couple of coefficient  $(c_{AV}, c_{\phi A})$  varying  $\sqrt{s}$ .

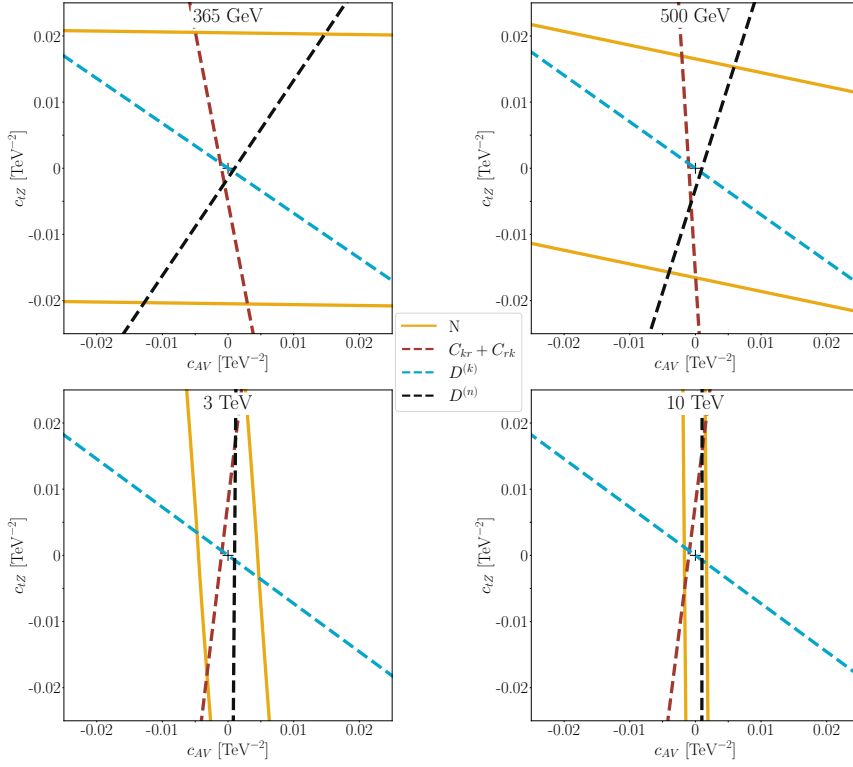

**Figure 12:** Exclusion plot for the couple of coefficient  $(c_{AV}, c_{tZ})$  varying  $\sqrt{s}$ .

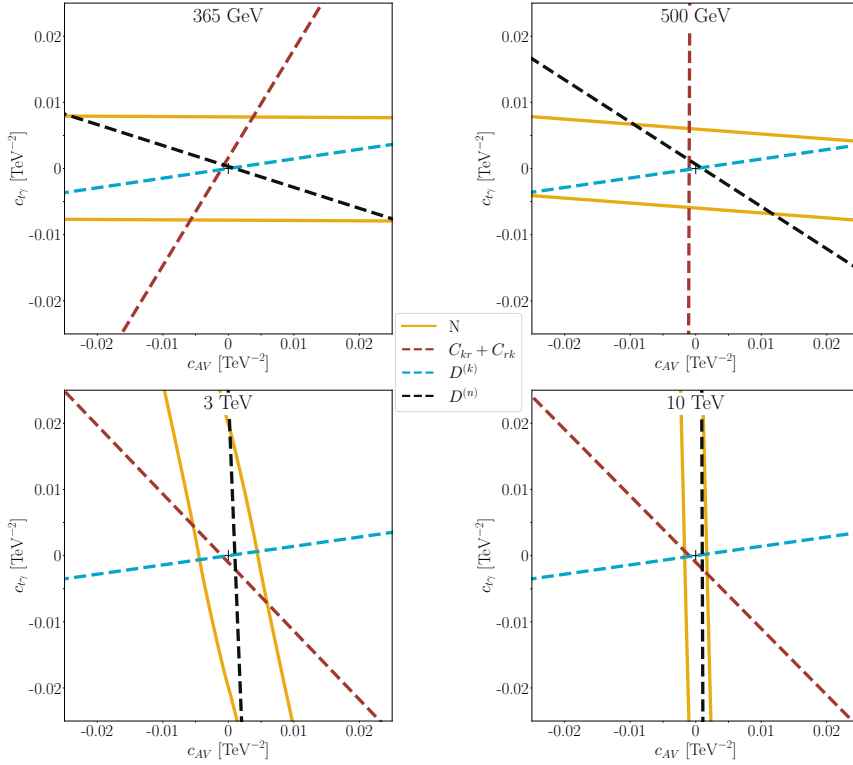

**Figure 13:** Exclusion plot for the couple of coefficient  $(c_{AV}, c_{t\gamma})$  varying  $\sqrt{s}$ .

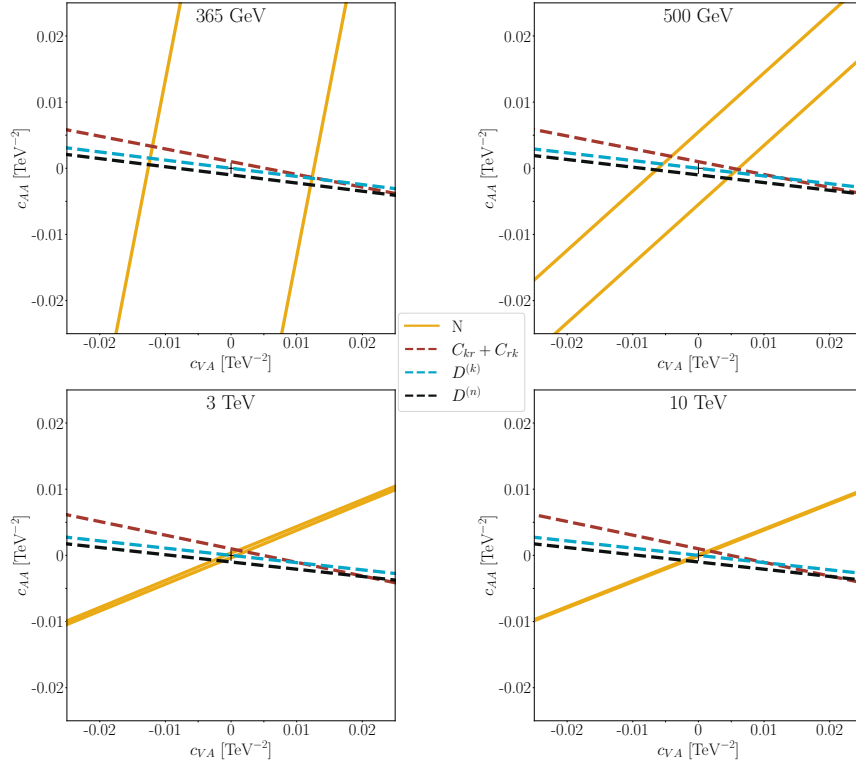

**Figure 14:** Exclusion plot for the couple of coefficient  $(c_{VA}, c_{AA})$  varying  $\sqrt{s}$ .

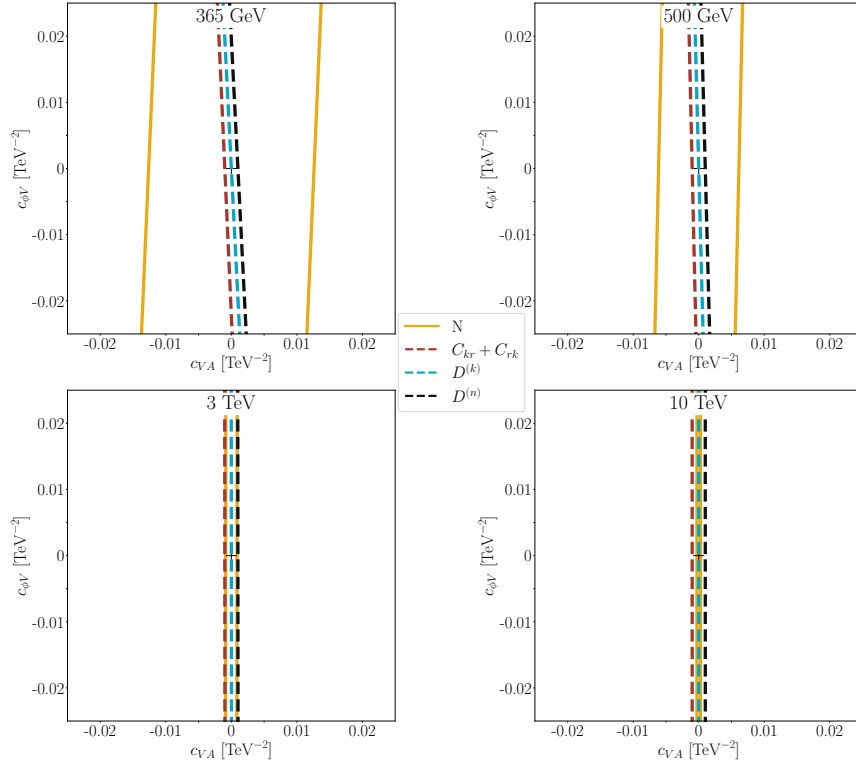

**Figure 15:** Exclusion plot for the couple of coefficient  $(c_{VA}, c_{\phi V})$  varying  $\sqrt{s}$ .



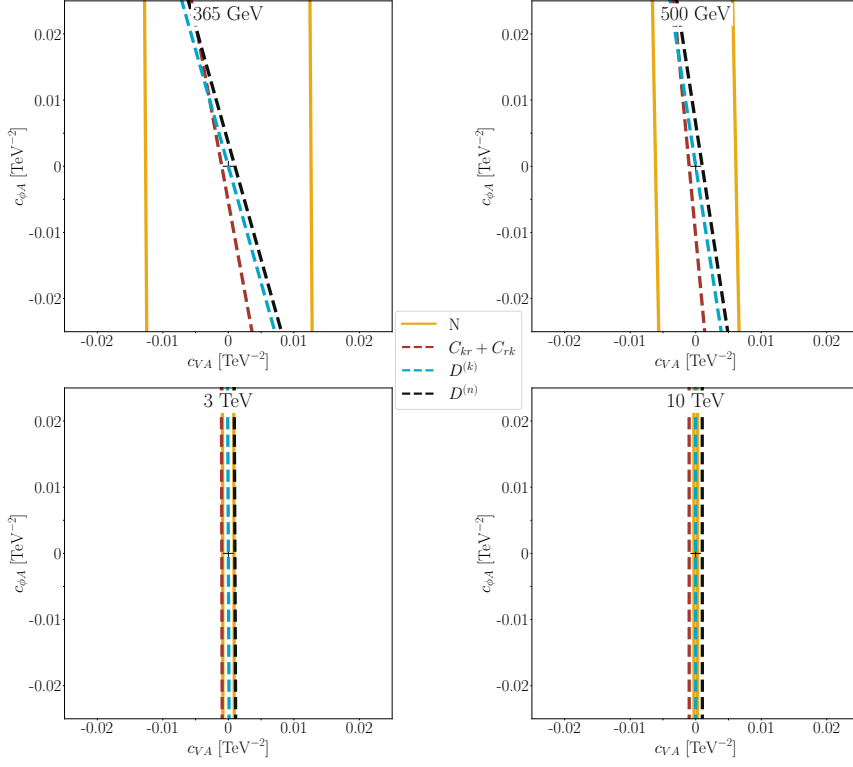

**Figure 16:** Exclusion plot for the couple of coefficient  $(c_{VA}, c_{\phi A})$  varying  $\sqrt{s}$ .

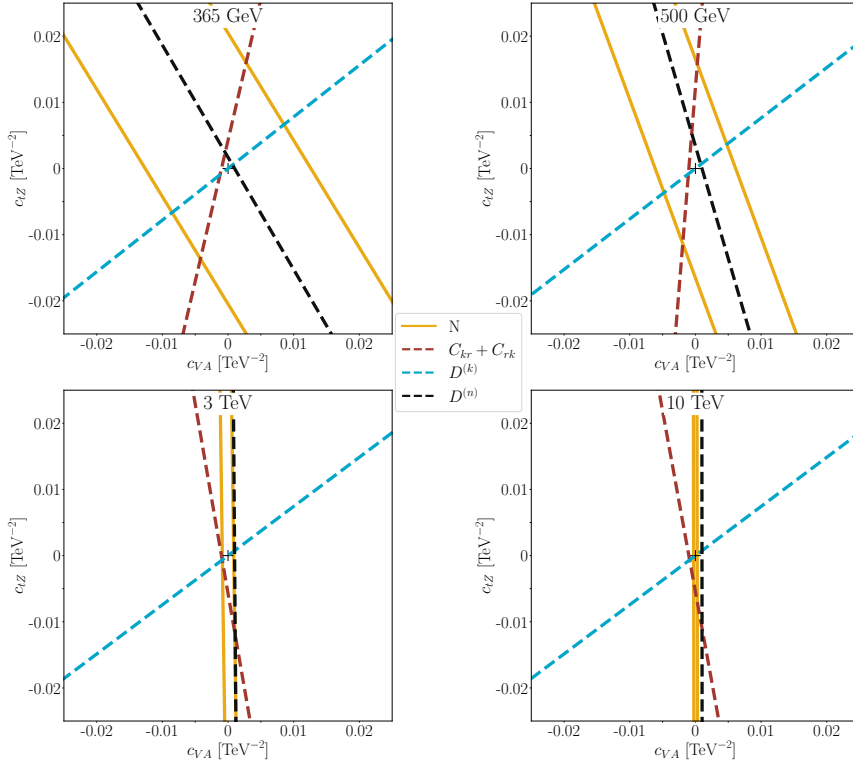

**Figure 17:** Exclusion plot for the couple of coefficient  $(c_{VA}, c_{tZ})$  varying  $\sqrt{s}$ .

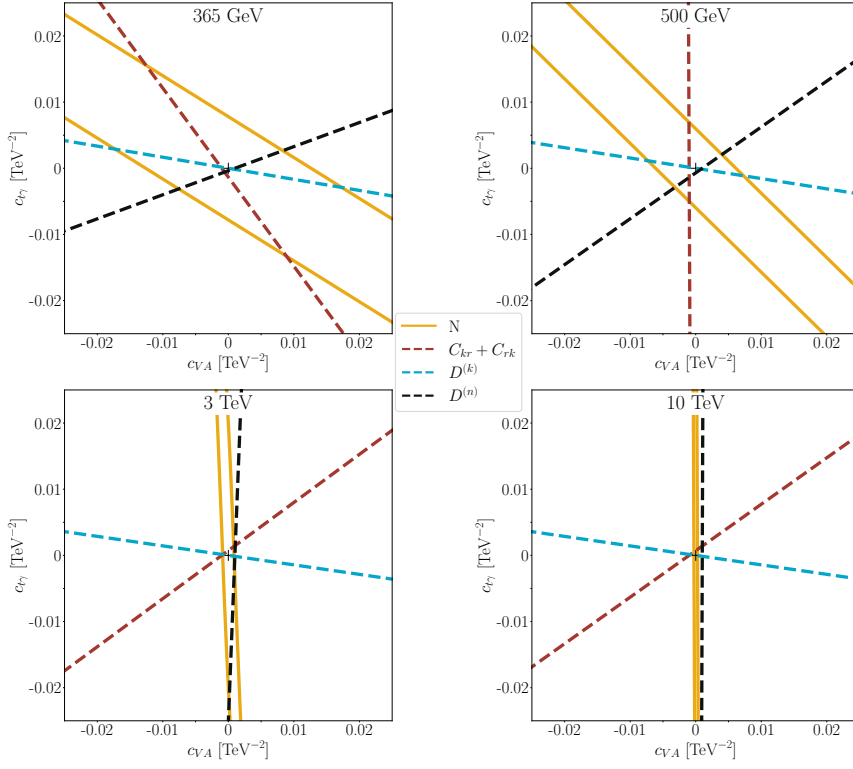

**Figure 18:** Exclusion plot for the couple of coefficient  $(c_{VA}, c_{t\gamma})$  varying  $\sqrt{s}$ .

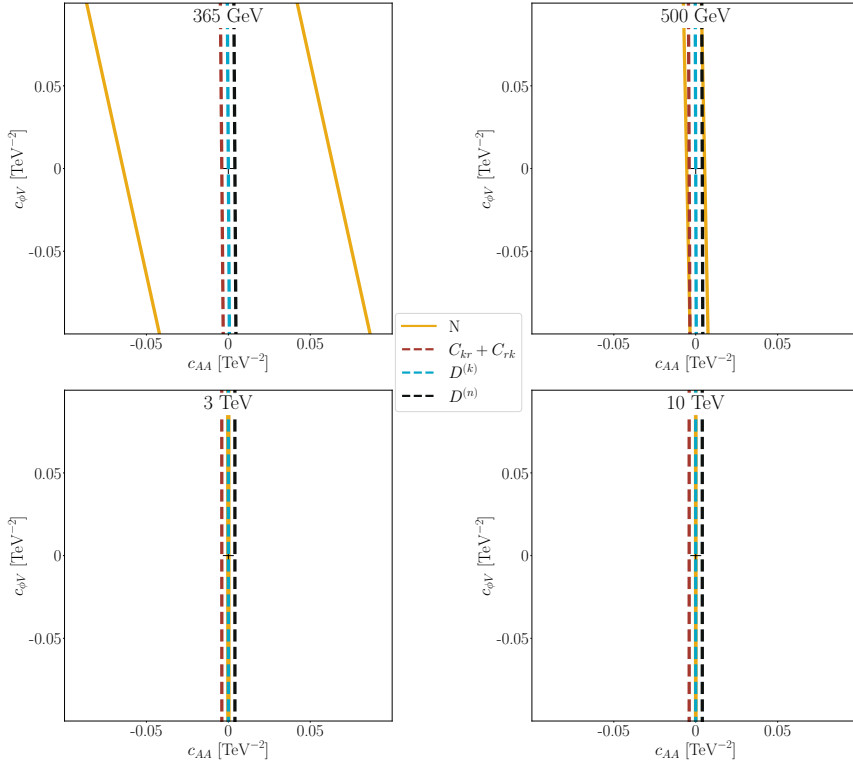

**Figure 19:** Exclusion plot for the couple of coefficient  $(c_{AA}, c_{\phi V})$  varying  $\sqrt{s}$ .

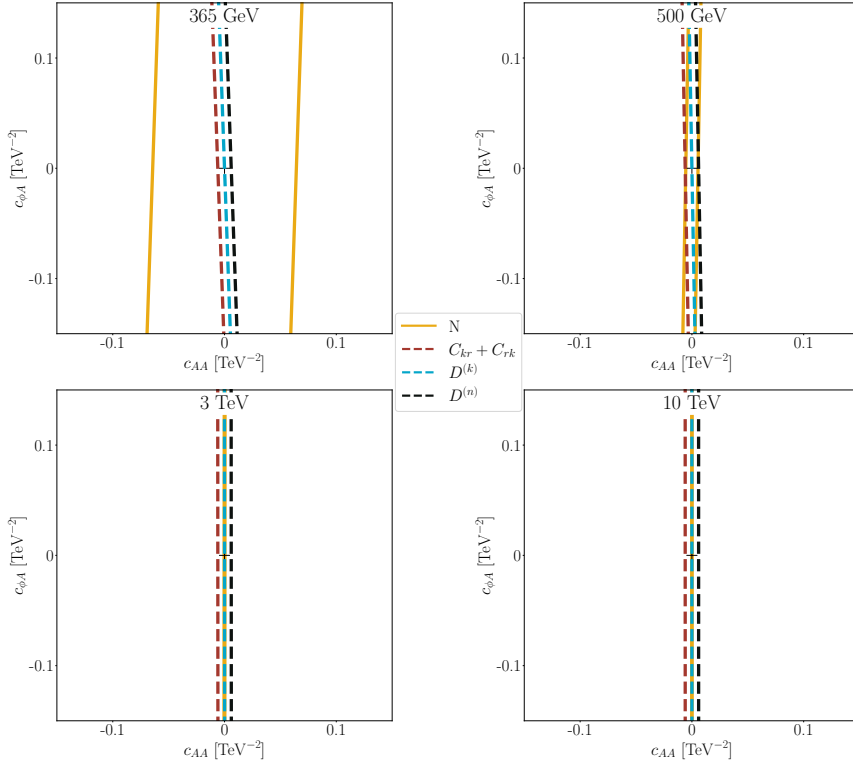

**Figure 20:** Exclusion plot for the couple of coefficient  $(c_{AA}, c_{\phi A})$  varying  $\sqrt{s}$ .

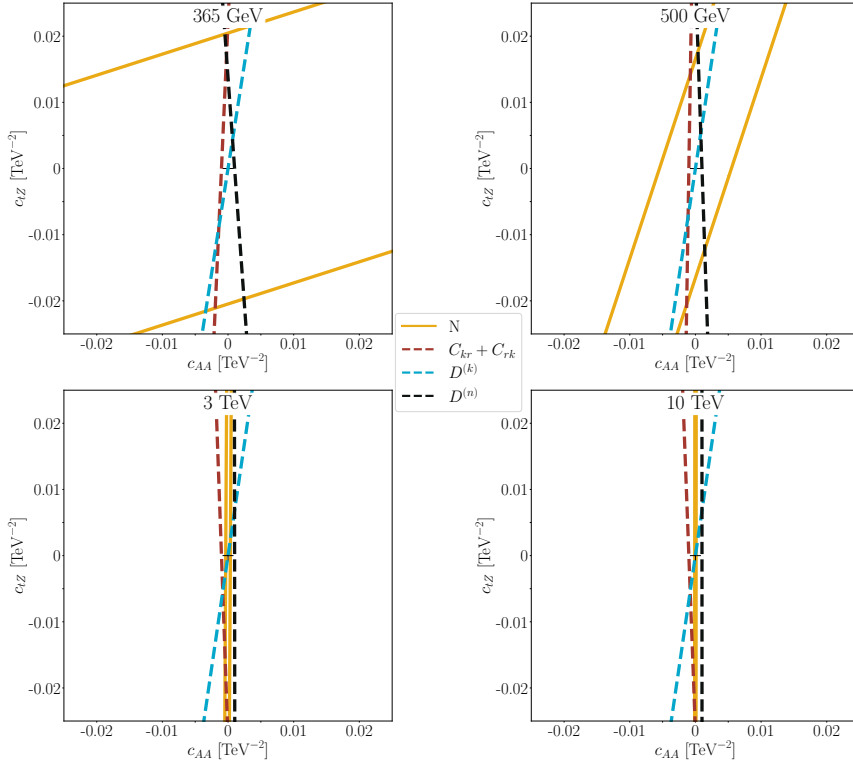

**Figure 21:** Exclusion plot for the couple of coefficient  $(c_{AA}, c_{tZ})$  varying  $\sqrt{s}$ .

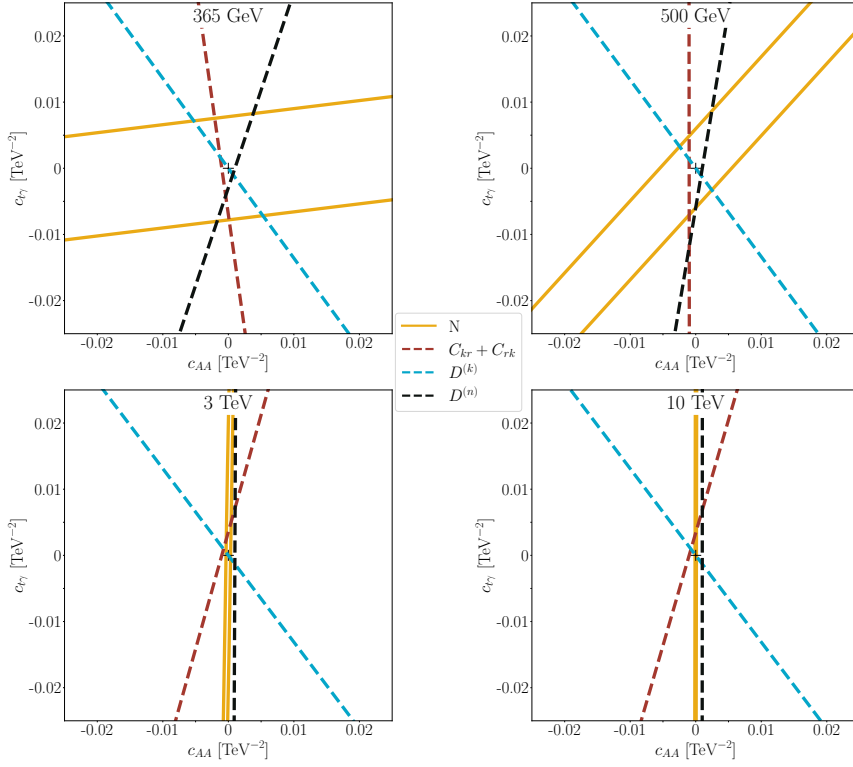

**Figure 22:** Exclusion plot for the couple of coefficient  $(c_{AA}, c_{t\gamma})$  varying  $\sqrt{s}$ .

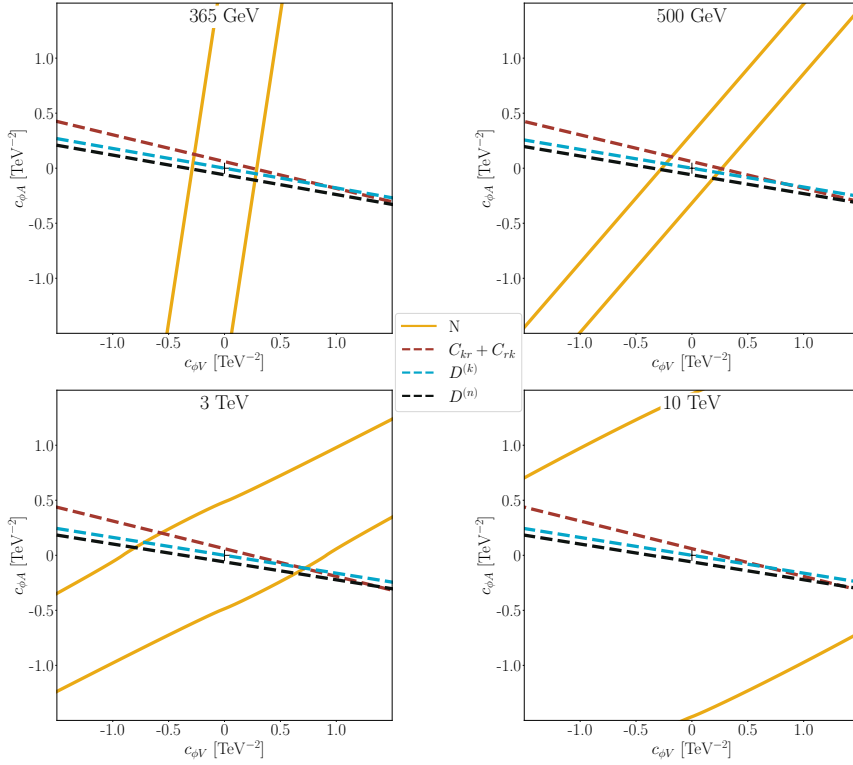

**Figure 23:** Exclusion plot for the couple of coefficient  $(c_{\phi V}, c_{\phi A})$  varying  $\sqrt{s}$ .

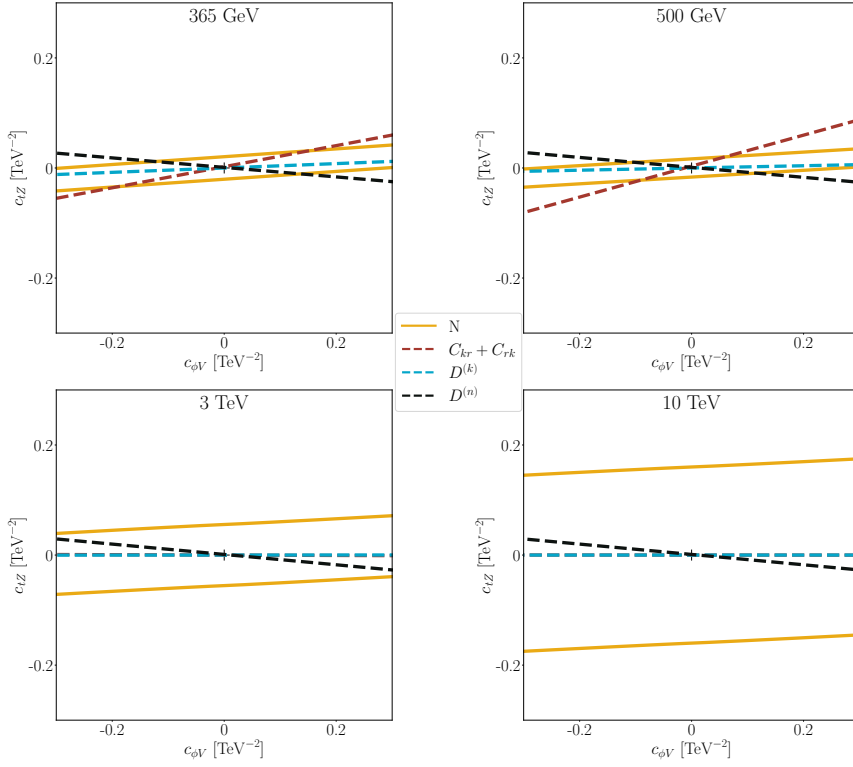

**Figure 24:** Exclusion plot for the couple of coefficient  $(c_{\phi V}, c_{tZ})$  varying  $\sqrt{s}$ .

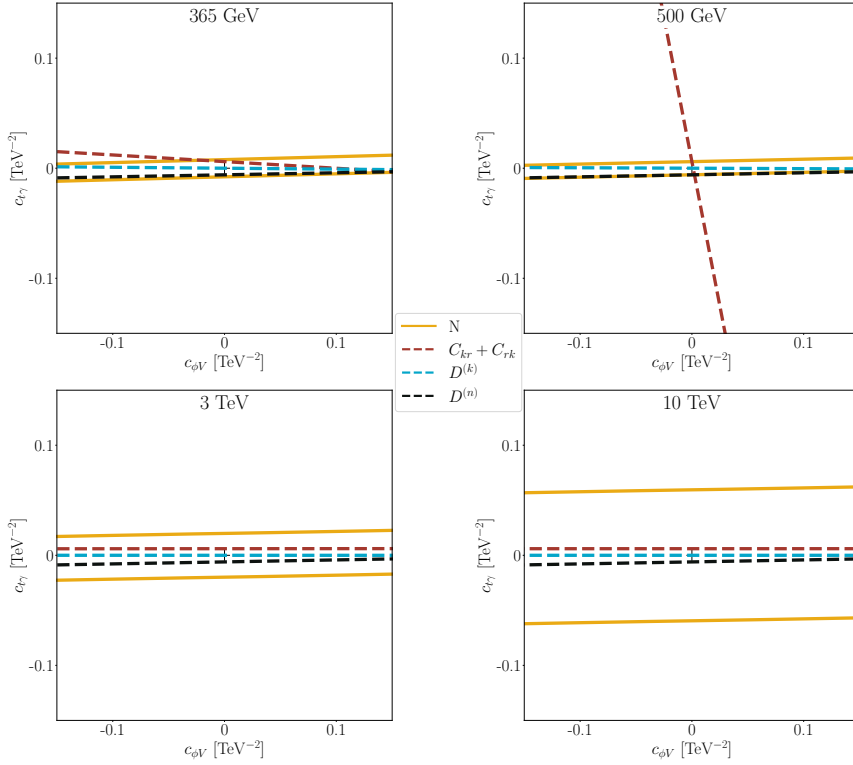

**Figure 25:** Exclusion plot for the couple of coefficient  $(c_{\phi V}, c_{t\gamma})$  varying  $\sqrt{s}$ .

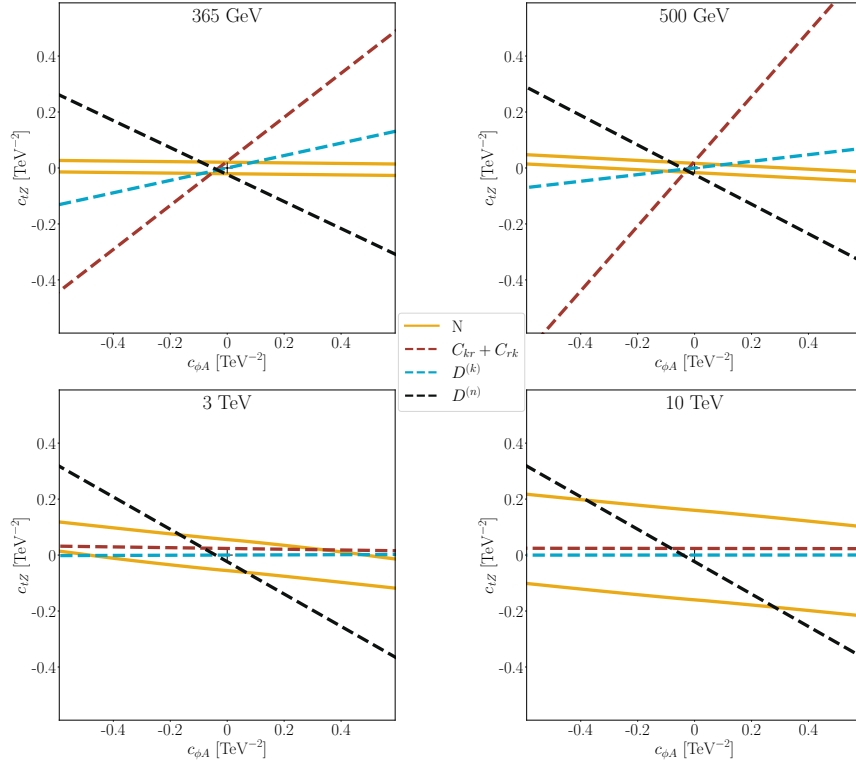

**Figure 26:** Exclusion plot for the couple of coefficient  $(c_{\phi A}, c_{tZ})$  varying  $\sqrt{s}$ .

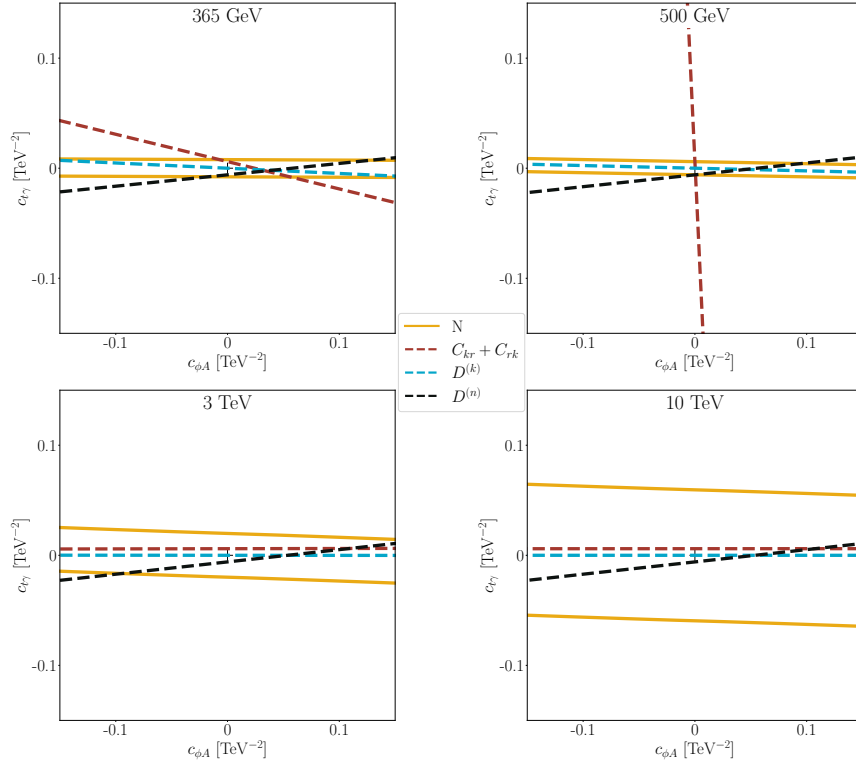

**Figure 27:** Exclusion plot for the couple of coefficient  $(c_{\phi A}, c_{t\gamma})$  varying  $\sqrt{s}$ .

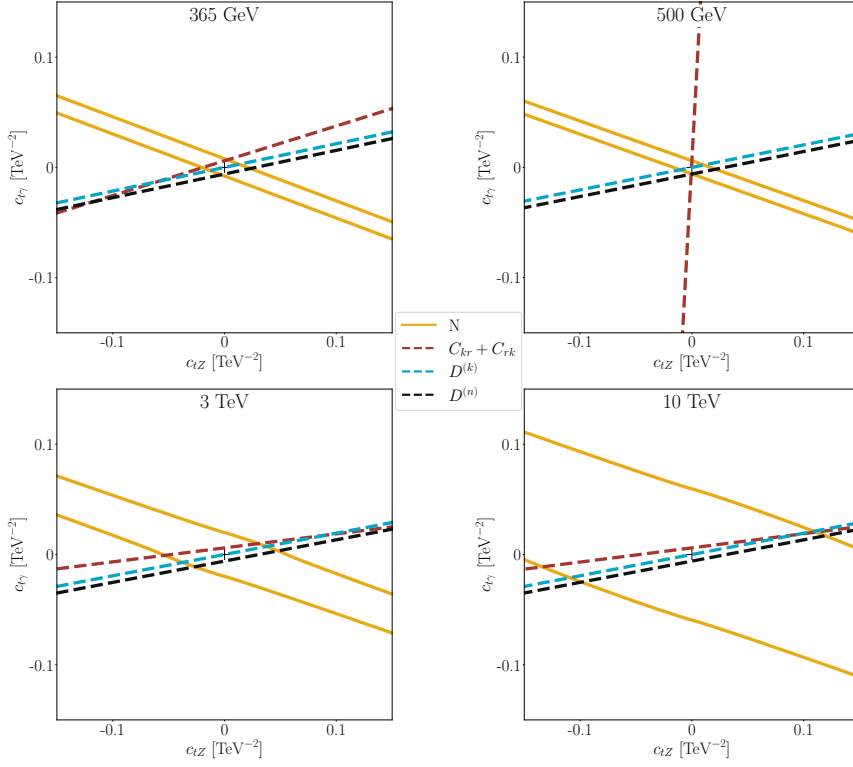

**Figure 28:** Exclusion plot for the couple of coefficient  $(c_{tZ}, c_{t\gamma})$  varying  $\sqrt{s}$ .
